# Supplementary material for: Probing quantum mechanics using nanoparticle Schr\"odinger cats
Source: arXiv:2507.21211 source file (2025-07-28)
Supplement: Supplementary file 1 [file Pedalino_2025_SI.pdf]

# Supplementary Information:
Probing quantum mechanics using nanoparticle Schrödinger cats

Sebastian Pedalino[1,2], Bruno E. Ramírez-Galindo[1,2], Richard Ferstl[1,2], Klaus Hornberger[3], Markus Arndt[1*], Stefan Gerlich[1]

[1]University of Vienna, Faculty of Physics, Boltzmanngasse 5, Vienna, 1090, Austria.
[2]University of Vienna, Vienna Doctoral School in Physics, Boltzmanngasse 5, Vienna, 1090, Austria.
[3]University of Duisburg-Essen, Faculty of Physics, Lotharstraße 1, Duisburg, 47048, Germany.

*Corresponding author(s). E-mail(s): markus.arndt@univie.ac.at;
Contributing authors: sebastian.pedalino@univie.ac.at;

## Contents

**1 Experiment** **2**
1.1 Details of the setup . . . 2
1.2 Velocity distribution . . . 2
1.3 Photo-ionization and mass selection . . . 3
1.4 High-mass fringes and ultraviolet polarizability . . . 4

**2 Phase averaging and decoherence** **4**
2.1 Gravity and the rotation of the Earth . . . 4
2.2 Interferometer vibrations . . . 5
2.3 Collisional decoherence . . . 5
2.4 Thermal and optical decoherence . . . 6

**3 Quantitative analysis** **6**

# 1 Experiment

## 1.1 Details of the setup

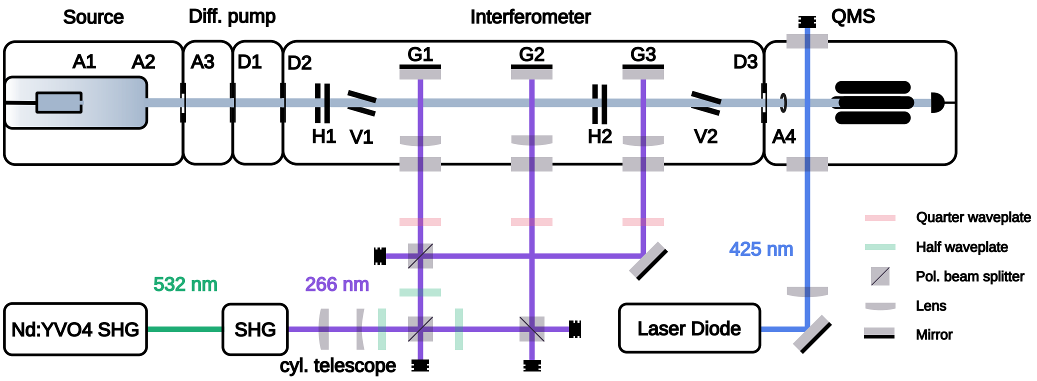


**Suppl. Fig. 1**: **Cluster beam apparatus and laser system.** The $D_i$ are apertures for differential pumping, $G_i$ are the diffraction gratings. H and V are horizontal and vertical delimiters for alignment. The second harmonic (SHG) of the green DPSS laser light is shaped by a cylindrical telescope and focused by three cylindrical lenses to achieve a small waist ($20\,\mu$m) in the direction of the cluster beam.

In Suppl. Figure 1 we show details of the experimental setup, including vacuum chambers, differential pumping stages, and laser system: Sodium atoms are evaporated in an effusive source with aperture (A1) and aggregate to large clusters in the cryogenic noble gas chamber. They exit through a thin aperture (A2) of 5 mm diameter into the source chamber at $4.8 \times 10^{-3}$ mbar and pass another 5 mm diameter aperture (A3) into two differential pumping stages, each separated from the next by a vertical $1 \times 20\,\mathrm{mm}^2$ slit, D1 and D2. These stages are pumped to $4.3 \times 10^{-7}$ mbar and $5.0 \times 10^{-8}$ mbar, respectively. When the cluster beam is on, the interferometer chamber reaches a pressure of $8.5 \times 10^{-9}$ mbar. The detector chamber, separated by D3, is held at $8.5 \times 10^{-8}$ mbar. A pair of horizontal slits, H1 and H2, collimates the cluster beam and allows us to align it to each mirror yaw angle with a precision of 200 µrad. A pair of vertical collimation slits, V1 and V2, restricts the height of the cluster beam to keep it smaller than the vertical waist of the UV gratings. This allows treating the laser beam profile as homogeneous and to minimize the sensitivity to misalignment with respect to Earth's gravity [52].

The frequency-doubled DPSS laser beam at 266 nm is divided into three parts using polarization optics. To suppress back reflections into the laser, the standing light wave is circularly polarized. The helicity of the light field does not influence the diffraction phase, as the clusters do not have any specific direction or helicity, and they come with random orientation. All gratings are mounted on motorized horizontal translation stages. $G_2$ and the cylindrical focusing lens, 100 mm in front of it, can additionally be vertically shifted, with nanometer resolution and over up to 1 cm in height, to compensate for the gravitational free fall of nanoparticles in different velocity classes.

## 1.2 Velocity distribution

The cluster velocity is measured in a time-of-flight setting, where the start signal is given by the interruption of an ionizing UV photodepletion beam and the stop signal is the arrival time at the detector. In Suppl. Figure 2a, we show a typical time-of-flight curve, while panel (b) shows the velocity that is derived from it by transforming $f(t)\mathrm{d}t \to f(v)\mathrm{d}v$. We also account for the slight acceleration of the ions within the quadrupole mass spectrometer, which modifies the total transit time.

$$t_d = \frac{L}{v_0} + \frac{L_\mathrm{Q}}{\sqrt{v_0^2 + 2qU/m}}. \tag{1}$$

Here, $L = (2.74 \pm 0.03)$ m is the neutral drift length in the interferometer, $L_\mathrm{Q} = (0.30 \pm 0.05)$ m is the length of the mass filter, and $U \simeq 9$ V the acceleration voltage in the filter. The finite opening time of the photodepletion laser is accounted for by fitting a convolution of the opening function and a Gaussian time distribution to the denoised data. In several different runs, we find a mean velocity around 160 m/s, and a full width at half maximum (FWHM) of typically 10 m/s, see Suppl. Figure 2. In every run, the velocity is reconfirmed.

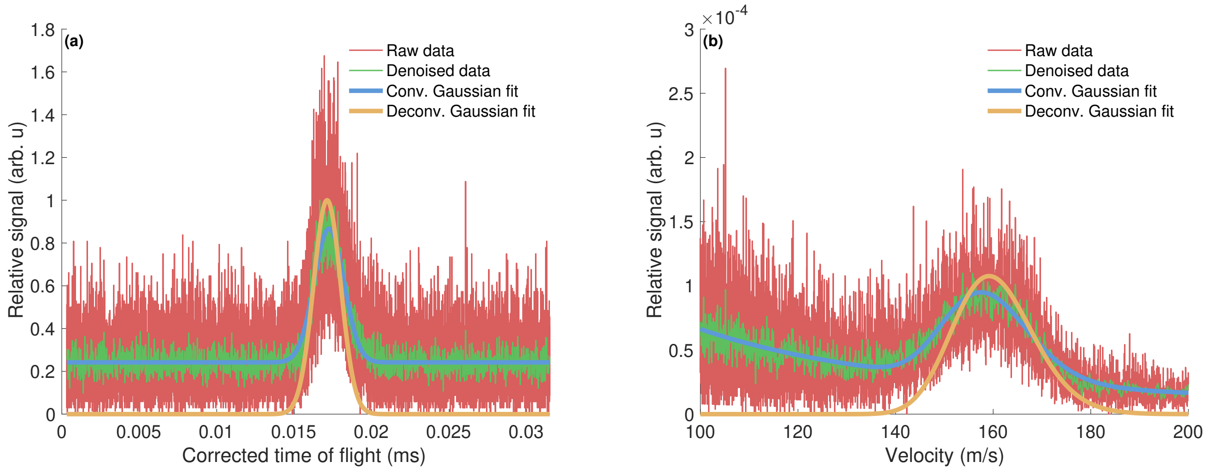


**Suppl. Fig. 2**: **Velocity distributions: (a)** Raw (light blue) and denoised (dark blue) time-of-flight data for 100 kTh clusters. We show the Gaussian drift time (purple) and the convoluted fit to the data (green). **(b)** Velocity distribution extracted from panel (a). The red line marks the mean of the convoluted Gaussian fitted to the data (shown in purple).

## 1.3 Photo-ionization and mass selection

Sodium has a low work function ($W = 2.75\,\text{eV}$) [53], which allows for sequential photon absorption and stepwise ionization. This process continues until the ionization energy of the cluster in charge state $z$ exceeds the photon energy $E_\gamma = h\nu$:

$$E_i[eV] = W + \frac{e(\alpha + z)}{4\pi\epsilon_0 r}. \tag{2}$$

The correction factor $\alpha \simeq 3/8$ accounts for surface effects [54].

Clusters of lower density $\rho$ have a larger radius $r$ and higher charge numbers can be attained. Sodium clusters with $\rho = 980\,\text{kg}\,\text{m}^{-3}$ and 200 kDa can therefore be ionized manifold for $\lambda = 266\,\text{nm}$. This does not affect the function of our photo-depletion gratings, as every ion is removed from the beam, independent of its charge state. However, it must be avoided in the detection process to avoid charge mixing.

Additionally, the detected signal $S$ is influenced by the dependence of the work function on temperature $T_{\text{cl}}$ and surface purity. To account for such effects, we have measured the cluster work function $W$ under conditions identical to those prevailing in the interference experiments, using wavelengths between $430 - 504\,\text{nm}$ and Fowler's law to analyze the data [55] :

$$\ln\left[\frac{S}{T_{\text{cl}}^2}\right] = B + \ln\left[\text{Li}_2\left(\frac{h\nu - W}{k_B T_{\text{cl}}}\right)\right]. \tag{3}$$

Here, $B$ is a material-specific fit constant, and the polylogarithmic function is

$$\text{Li}_2(z) = -\int_0^z \frac{\ln(1-t)}{t}\text{d}t \quad \text{for } |z| \leq 1. \tag{4}$$

Suppl. Figure 3a shows the experimental data along with a Fowler fit. Assuming the cluster temperature to be in equilibrium with the collisional bath in the source, the fit yields a work function of $W = (2.4 \pm 0.1)\,\text{eV}$. This low value of $W$ is consistent with some oxygen contamination. Based on this value, we expect to find at most doubly charged clusters when using a detection laser wavelength of $\lambda = 425\,\text{nm}$.

To verify this, we have first recorded a mass spectrum at low laser power $P_{\text{L}} = 15$ mW. This avoids double ionization across the entire accessible mass range and allows us to identify the smallest and the highest masses in the spectrum, see Suppl. Figure 3b. To increase the signal, we then switch to $P_{\text{L}} = 650$ mW, where double ionization dominates while triple ionization remains energetically inaccessible. In the low-power spectrum (blue) of panel (b), singly ionized clusters with masses below 100 kDa are essentially absent. Therefore, the left flank must be due to doubly ionized clusters. This allows us to assign $m/z \lesssim 100\,\text{kTh}$ in the high-power spectrum (red) to be confidently assigned to twice the measured $m/z$ value. The dashed line in the same panel shows a modeled high-power spectrum with a maximum charge state of +2, based on the assumption that the low-power spectrum is singly charged. It aligns well with our observed high-power spectrum.

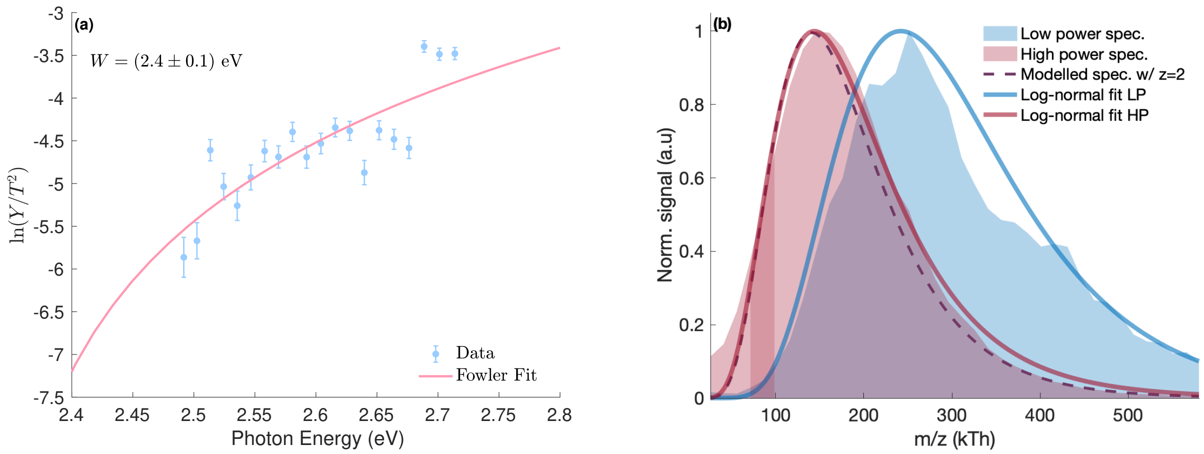


**Suppl. Fig. 3**: **(a) Na-Cluster ion signal as function of the photon energy.** Clusters with a diameter of $d \sim 8$ nm were ionized by the light of an optical parametric oscillator (Ekspla OPO, 100 Hz, 5 ns, $E \simeq 200 - 400\,\mu$J) The data (blue circles) are analyzed using a Fowler fit, shown as a solid red line. We fit $W = (2.4 \pm 0.1)$ eV. **(b) Mass spectra of sodium clusters**. The cluster beam is photo-ionized with 425 nm light at 15 mW (blue area) and 650 mW (red area). At low laser power, the clusters are only singly ionized, while they dominate in the 2+ state at high laser power. For interference experiments we use the left flank of the high-power spectrum. A model based on a log-normal size distribution (red and blue solid line) and size-dependent ionization probability reproduces the experimental data very well (dashed line). The spectrum corresponds to the interference scans in the main text, with the center mass marked as a dark vertical stripe at $m/z = 85$ kTh.

### 1.4 High-mass fringes and ultraviolet polarizability

The grating separation of our Talbot-Lau interferometer, $L = 0.983\,\mathrm{m} > L_T = d^2/\lambda_{\mathrm{dB}}$ defines the smallest usable de Broglie wavelength and thus the greatest cluster mass for the given velocity of 160 m/s. For shorter wavelengths, wave mechanics transitions into geometric optics. In this limit the interaction with grating $G_2$ is then fully determined by the quantities (see Methods)

$$\zeta_{\mathrm{coh}}(\xi) \simeq \phi_0 \pi \xi. \tag{5}$$

$$\zeta_{\mathrm{ion}} \simeq n_0/2 \tag{6}$$

which coincides with the classical prediction. The value of $n_0$ can be determined by the grating transmission, leaving only the product $\phi_0 \xi$ as a free parameter. It depends only on the product of laser power divided by velocity, the total cluster polarizability, and $\xi \equiv L/L_T \propto 1/m$. This means that $\zeta_{\mathrm{coh}}(\xi)$ becomes effectively independent of mass if the total polarizability scales linearly with $m$ and the velocity is independent of it.

A fit of the model to the measured fringe visibilities therefore provides a robust method for extracting the optical polarizability per atom without the need to know the precise mass distribution and without needing to distinguish between quantum and classical effects.

We find a fringe visibility of $V \simeq 0.66 \pm 0.09$ for clusters within $0.4 - 1.0$ MDa and use the $G_2$ power dependence $V(P_2)$ to extract the polarizability $\alpha_{266}/\mathrm{atom} = -4\pi\varepsilon_0 \times (4.5 \pm 0.5)\,\text{Å}^3$. This value is applied to model the interference scans of all clusters, both quantum mechanically and using classical theory.

## 2 Phase averaging and decoherence

### 2.1 Gravity and the rotation of the Earth

The interference fringes are shifted in the presence of the Earth's gravity and rotation. For an appropriate choice of the grating roll angles, both accelerations cancel to first order [56]. We estimate a contrast reduction factor $R > 0.99$ from these effects for the velocity distribution in our experiment.

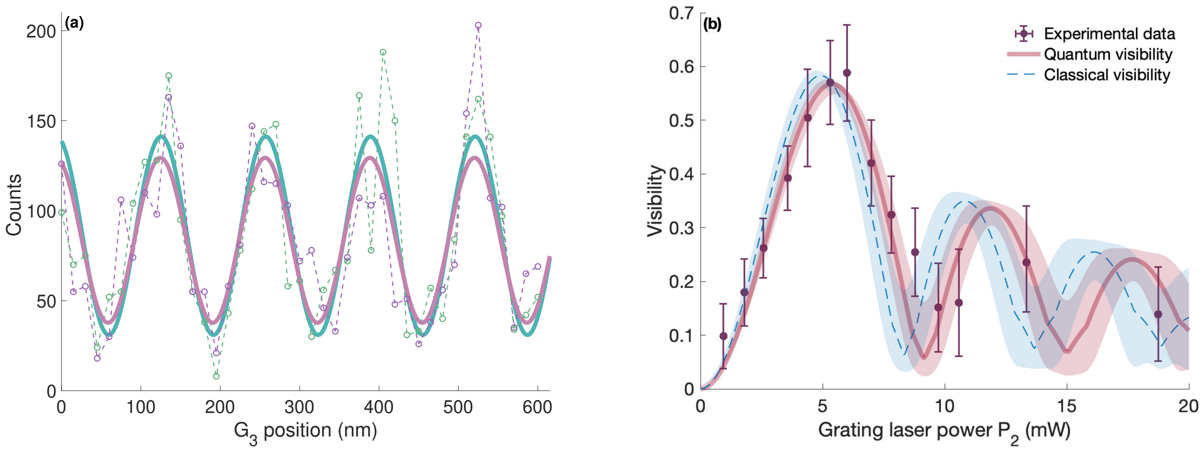


**Suppl. Fig. 4**: **(a) Fringe pattern of high-mass sodium clusters.** The contributing masses range between 0.4 MDa and 1.0 MDa. The grating laser powers are $P_1 = P_3 = (60\pm5)$ mW and $P_2 = (6.2\pm0.5)$ mW. Sinusoidal fits to the experimental data (circles) identify a visibility of $V = 0.66 \pm 0.09$ (green line) and $V = 0.56 \pm 0.10$ (red line). **(b) Fringe visibility as a function of the grating laser power in $\mathbf{G_2}$.** $P_{1,3}$ and the masses are like in panel (a). The experimental data (purple circles) are equally well described by the quantum (red solid line) and the classical (blue dashed line) prediction. The shaded areas represent the effect of known uncertainties in the cluster velocity in the model. We extract the polarizability per atom from a fit to the model and find $\alpha_{266}/\text{atom} = -4\pi\varepsilon_0 \times (4.5 \pm 0.5)\,\text{Å}^3$.

## 2.2 Interferometer vibrations

Grating vibrations can reduce the fringe visibility by

$$R_0 = |\langle \exp\left[i2\pi(\Delta x_1 - 2\Delta x_2 + \Delta x_3)/d\right]\rangle|, \tag{7}$$

where $\langle\cdot\rangle$ indicates the ensemble average over all grating shifts.

When sinusoidal vibrations across a broad frequency spectrum add randomly varying amplitudes and frequencies, one can model the displacements $\Delta x_i, (i = 1, 2, 3)$ as a stochastic variable with normal distribution. If the root mean squared amplitude $\Delta x_{\text{RMS}}$ is the same in all three gratings, the contrast reduction factor is

$$R_V = \left|\exp\left(-8\pi^2\Delta x^2_{\text{RMS}}/d^2\right)\right|. \tag{8}$$

In order to minimize vibrations, all gratings are mounted on motorized stages on a single 160 kg Invar bar that is suspended by four piano wires from an aluminum gallows supported by four springs. Additionally, Teflon balls between stacks of steel and eddy current brakes contribute to isolation and damping. The entire vacuum chamber is mounted on an optical table (resonance frequency 2 Hz) which floats on pneumatic feet [56].

We monitor the vibrations using a tri-axial accelerometer (PCB 356M98) on the Invar bar and find the vibration amplitude to lie below the accelerometer noise floor. This level of isolation is compatible with the observed fringe visibility: An average grating vibration as small as $\Delta x_{\text{RMS}} \simeq 7$ nm could by itself explain the observed total contrast reduction factor – even in the absence of any other decoherence or phase averaging mechanism.

## 2.3 Collisional decoherence

The interferometer chamber is pumped by four turbo molecular pumps (Pfeiffer Hi-Pace 700), two combined ion getter and titanium sublimation pumps (Varian VacIon Plus 300 Combination) as well as two non-evaporable getter pumps (SAES Capacitorr Z1000). It is separated from the source and detection chamber by three differential pumping stages. This ensures a base pressure of $4 \times 10^{-9}$ mbar and below $9 \times 10^{-9}$ mbar during the operation of the cluster source.

Collisions can decohere the interference contrast if the clusters remain within the detection angle. We then expect a reduction factor $R_c = \exp\left(-2\Gamma_c T\right)$ that scales with the time in the interferometer, $2T$, and the collision

rate $\Gamma_c$, which is dominated by van der Waals interactions [57, 58]:

$$\Gamma_c \approx \frac{8p_g}{k_\mathrm{B}T_g}\left(\frac{C_6^2 v_g^3}{\hbar^2}\right)^{1/5}. \tag{9}$$

Here $p_g$, $T_g$, and $v_g$ are the pressure, temperature, and most probable velocity of the background gas, respectively. The coefficient $C_6$ can be estimated using the Slater-Kirkwood formula [58].

$$C_6 \approx \frac{3}{2}\frac{e\hbar}{\sqrt{m_e}(4\pi\varepsilon_0)^2}\frac{\bar{\alpha}_g\bar{\alpha}}{\sqrt{\bar{\alpha}_g/N_g}+\sqrt{\bar{\alpha}/N}} \tag{10}$$

The expected contrast reduction at our measured pressure $p_g = 9\times10^{-9}$ mbar and $T_c = 300$ K then depends on the partial pressure in the chamber at the time of the measurement. While we did not have a calibrated rest gas analyzer inside the interferometer chamber, a model distribution composed of $4.6\times10^{-9}$ mbar ($H_2O$), $1.4\times10^{-9}$ mbar (He) and $3\times10^{-9}$ mbar ($H_2$) [59] for our unbaked chamber is sufficient to explain an experimental visibility reduction factor of $R_c = 0.79$. Because of its high velocity, $H_2$ is the most detrimental and was estimated to have a larger contribution here to give a lower bound for $R_c$.

For this estimate we use the static polarizability of bulk sodium $\bar{\alpha}/N_\mathrm{atoms} = 4\pi\varepsilon_0\times 9.4\,\text{Å}^3$ and one valence electron per atom $N = N_\mathrm{atoms}$. The rest gas polarizabilities and valence numbers are $\bar{\alpha}_g = 4\pi\varepsilon_0\times0.8\,\text{Å}^3$, $N_g = 2$ for $H_2$, $\bar{\alpha}_g = 4\pi\varepsilon_0\times1.5\,\text{Å}^3$, $N_g = 8$ for $H_2O$ and $\bar{\alpha}_g = 4\pi\varepsilon_0\times0.2\,\text{Å}^3$, $N_g = 2$ for He [60].

### 2.4 Thermal and optical decoherence

In general, absorption, scattering, and emission of thermal radiation can reduce the cluster interference contrast [61]. However, for the internal temperature (ca. 80 K) of our clusters, we do not expect any observable effect related to emission [62]. Similarly, Rayleigh scattering at the optical gratings and evaporation of individual sodium atoms can be neglected [63].

## 3 Quantitative analysis

In Suppl. Figure 5, we present the unscaled visibilities as a function of the $G_2$ grating laser power, comparing the results to predictions from both the classical and quantum models. The visibilities were derived from sinusoidal fits of the raw interference scans.

In Suppl. Figure 6 we provide the final posterior of the classicalization time distribution (blue line), which determines the macroscopicity reached in the experiment (arrow). Jeffreys' prior (dashed line) and intermediate posteriors (black lines) are shown as well.

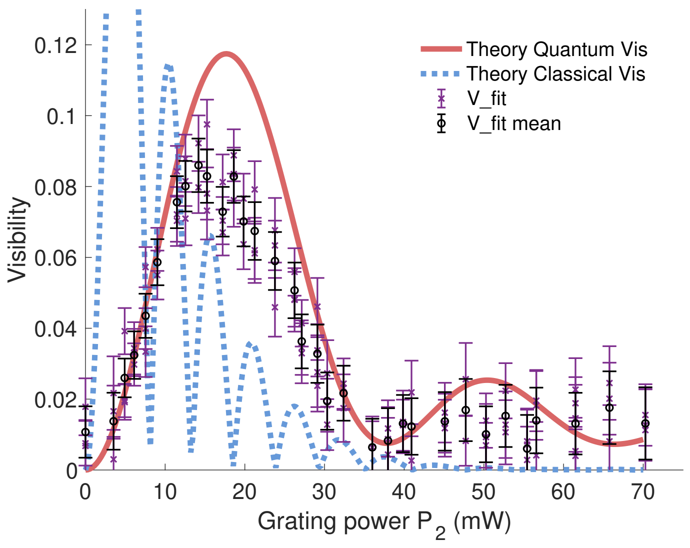


**Suppl. Fig. 5**: We show the measured raw visibilities together with the unscaled classical (red dashed line) and quantum fringe visibility (black line) as a function of laser power in $G_2$ for $m_0 = 172$ kDa.

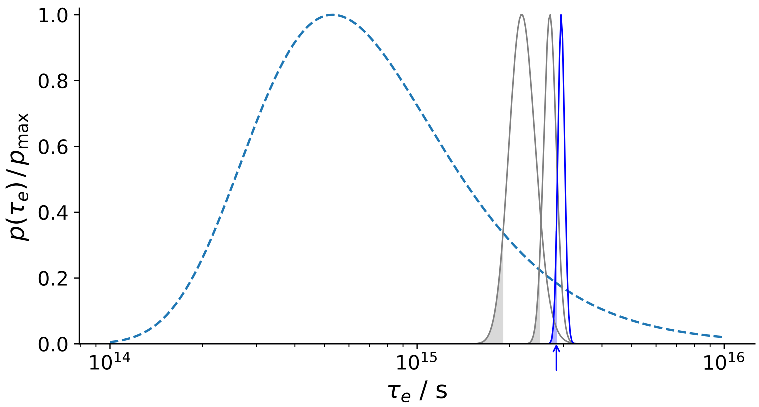


**Suppl. Fig. 6**: **Probability distributions $p(\tau_e)$ of the classicalization time.** The dashed line gives Jeffreys' prior, which is taken as a starting point. Bayesian updating yields posterior distributions from the recorded particle counts by means of the MMM likelihoods, calculated for the different lateral positions $x_3$ and grating powers $P_2$ with $\hbar/\sigma_q = 10\,\mathrm{nm}$. The grey lines give intermediate posterior distributions after 123 counts (left) and 410 counts (right), corresponding to 4 and 10 grating scans. The blue line gives the final posterior distribution after 95 scans (3895 data points). The shaded areas indicate the 5% quantiles, finally located at $\tau_e = 2.84 \times 10^{15}\,\mathrm{s}$ (arrow). This value remains constant to three decimals as the last 15 scans are included.

In Figure 4a of the main text, we compare macroscopicity values for a selection of quantum experiments. They were provided by [64–67] or estimated in the original works, as summarized in Suppl. Table 1.

| Experiment type | Year | Macroscopicity | Ref. |
|---|---|---|---|
| Atoms | 1988 | 6.8 | [68] |
| | 1992 | 9.1 | [69] |
| | 1999 | 8.3 | [70] |
| | 2015 | 10.9 | [71] |
| | 2017 | 12.4 | [72] |
| | 2019 | 11.8 | [73] |
| BECs | 1997 | 8.4 | [74] |
| | 2013 | 8.5 | [75] |
| Mech. Resonators | 2018 | 7.8 | [76] |
| | 2022 | 11.2 | [77] |
| Molecules | 1995 | 7.2 | [78] |
| | 1999 | 10.6 | [79] |
| | 2009 | 10.9 | [80] |
| | 2013 | 12.3 | [81] |
| | 2019 | 14.0 | [82] |

**Suppl. Table 1**: References for the macroscopicity values of selected quantum experiments values shown in Figure 4a of the main text.

# References


[52] Pedalino, S., Ramirez Galindo, B., Sousa, T., Fein, Y.F., Geyer, P., Gerlich, S., Arndt, M.: Experimental challenges for high-mass matter-wave interference with nanoparticles. SPIE, Quant. Sens., Imag. and Prec. Metrol. **12447**, 1–10 (2023) https://doi.org/10.1117/12.2657260

[53] Wong, K., Tikhonov, G., Kresin, V.V.: Temperature-dependent work functions of free alkali-metal nanoparticles. Phys. Rev. B **66**, 125401 (2002) https://doi.org/10.1103/PhysRevB.66.125401

[54] De Heer, W.A.: The physics of simple metal clusters: Experimental aspects and simple models. Rev. Mod. Phys. **65**, 611–676 (1993) https://doi.org/10.1103/RevModPhys.65.611

[55] Fowler, R.H.: The analysis of photoelectric sensitivity curves for clean metals at various temperatures. Phys. Rev. **38**(1), 45–56 (1931) https://doi.org/10.1103/PhysRev.38.45

[56] Fein, Y.Y., Kiałka, F., Geyer, P., Gerlich, S., Arndt, M.: Coriolis compensation via gravity in a matter-wave interferometer. New J. Phys. **22**, 033013 (2020) https://doi.org/10.1088/1367-2630/ab73c5

[57] Hornberger, K., Uttenthaler, S., Brezger, B., Hackermüller, L., Arndt, M., Zeilinger, A.: Collisional decoherence observed in matter wave interferometry. Phys. Rev. Lett. **90**, 160401 (2003) https://doi.org/10.1103/PhysRevLett.90.160401

[58] Kiałka, F., Fein, Y.Y., Pedalino, S., Gerlich, S., Arndt, M.: A roadmap for universal high-mass matter-wave interferometry. AVS Quant. Sci. **4**, 020502 (2022) https://doi.org/10.1116/5.0080940

[59] Dobrozemsky, R.: Experience with a Computer Program for Residual Gas Analyzers. Journal of Vacuum Science and Technology **9**(1), 220–223 (1972) https://doi.org/10.1116/1.1316559

[60] Olney, T.N., Cann, N.M., Cooper, G., Brion, C.E.: Absolute scale determination for photoabsorption spectra and the calculation of molecular properties using dipole sum-rules. Chemical Physics **223**(1), 59–98 (1997) https://doi.org/10.1016/S0301-0104(97)00145-6

[61] Hackermüller, L., Hornberger, K., Brezger, B., Zeilinger, A., Arndt, M.: Decoherence of matter waves by thermal emission of radiation. Nature **427**, 711–714 (2004) https://doi.org/10.1038/Nature02276

[62] Schäfer, J., Stickler, B.A., Hornberger, K.: Decoherence of dielectric particles by thermal emission. Physical Review Research **6**(4), 043307 (2024) https://doi.org/10.1103/PhysRevResearch.6.043307

[63] Schäfer, J., Stickler, B.A., Hornberger, K.: Desorption-Induced Decoherence of Nanoparticle Motion. arXiv (2025). https://doi.org/10.48550/arXiv.2503.05475

[64] Nimmrichter, S., Hornberger, K.: Macroscopicity of Mechanical Quantum Superposition States. Physical Review Letters **110**(16), 160403 (2013) https://doi.org/10.1103/PhysRevLett.110.160403

[65] Schrinski, B., Yang, Y., Von Lüpke, U., Bild, M., Chu, Y., Hornberger, K., Nimmrichter, S., Fadel, M.: Macroscopic Quantum Test with Bulk Acoustic Wave Resonators. Physical Review Letters **130**(13), 133604 (2023) https://doi.org/10.1103/PhysRevLett.130.133604

[66] Schrinski, B., Nimmrichter, S., Stickler, B.A., Hornberger, K.: Macroscopicity of quantum mechanical superposition tests via hypothesis falsification. Physical Review A **100**(3), 032111 (2019) https://doi.org/10.1103/PhysRevA.100.032111

[67] Schrinski, B., Nimmrichter, S., Hornberger, K.: Quantum-classical hypothesis tests in macroscopic matter-wave interferometry. Physical Review Research **2**(3), 033034 (2020) https://doi.org/10.1103/PhysRevResearch.2.033034

[68] Keith, D.W., Schattenburg, M.L., Smith, H.I., Pritchard, D.E.: Diffraction of Atoms by a Transmission Grating. Physical Review Letters **61**(14), 1580–1583 (1988) https://doi.org/10.1103/PhysRevLett.61.1580

[69] Shimizu, F., Shimizu, K., Takuma, H.: Double-slit interference with ultracold metastable neon atoms. Physical Review A **46**(1), 17–20 (1992) https://doi.org/10.1103/PhysRevA.46.R17

[70] Grisenti, R.E., Schöllkopf, W., Toennies, J.P., Hegerfeldt, G.C., Köhler, T.: Determination of Atom-Surface van der Waals Potentials from Transmission-Grating Diffraction Intensities. Physical Review Letters **83**(9), 1755–1758 (1999) https://doi.org/10.1103/PhysRevLett.83.1755

[71] Kovachy, T., Asenbaum, P., Overstreet, C., Donnelly, C.A., Dickerson, S.M., Sugarbaker, A., Hogan, J.M., Kasevich, M.A.: Quantum superposition at the half-metre scale. Nature **528**, 530–3 (2015) https://doi.org/10.1038/nature16155

[72] Asenbaum, P., Overstreet, C., Kovachy, T., Brown, D.D., Hogan, J.M., Kasevich, M.A.: Phase Shift in an Atom Interferometer due to Spacetime Curvature across its Wave Function. Physical Review Letters **118**(18), 183602 (2017) https://doi.org/10.1103/PhysRevLett.118.183602

[73] Xu, V., Jaffe, M., Panda, C.D., Kristensen, S.L., Clark, L.W., Müller, H.: Probing gravity by holding atoms for 20 seconds. Science **366**(6466), 745–749 (2019) https://doi.org/10.1126/science.aay6428

[74] Andrews, M.R., Townsend, C.G., Miesner, H.-J., Durfee, D.S., Kurn, D.M., Ketterle, W.: Observation of Interference Between Two Bose Condensates. Science **275**(5300), 637–641 (1997) https://doi.org/10.1126/science.275.5300.637

[75] Berrada, T., Van Frank, S., Bücker, R., Schumm, T., Schaff, J.-F., Schmiedmayer, J.: Integrated Mach–Zehnder interferometer for Bose–Einstein condensates. Nature Communications **4**(1), 2077 (2013) https://doi.org/10.1038/ncomms3077

[76] Riedinger, R., Wallucks, A., Marinković, I., Löschnauer, C., Aspelmeyer, M., Hong, S., Gröblacher, S.: Remote quantum entanglement between two micromechanical oscillators. Nature **556**(7702), 473–477 (2018) https://doi.org/10.1038/s41586-018-0036-z

[77] Von Lüpke, U., Yang, Y., Bild, M., Michaud, L., Fadel, M., Chu, Y.: Parity measurement in the strong dispersive regime of circuit quantum acoustodynamics. Nature Physics **18**(7), 794–799 (2022) https://doi.org/10.1038/s41567-022-01591-2

[78] Chapman, M.S., Ekstrom, C.R., Hammond, T.D., Rubenstein, R.A., Schmiedmayer, J., Wehinger, S., Pritchard, D.E.: Optics and Interferometry with Na 2 Molecules. Physical Review Letters **74**(24), 4783–4786 (1995) https://doi.org/10.1103/PhysRevLett.74.4783

[79] Arndt, M., Nairz, O., Vos-Andreae, J., Keller, C., van der Zouw, G., Zeilinger, A.: Wave–particle duality of C60 molecules. Nature **401**(6754), 680–682 (1999) https://doi.org/10.1038/44348

[80] Hornberger, K., Gerlich, S., Ulbricht, H., Hackermüller, L., Nimmrichter, S., V Goldt, I., Boltalina, O., Arndt, M.: Theory and experimental verification of Kapitza–Dirac–Talbot–Lau interferometry. New Journal of Physics **11**(4), 043032 (2009) https://doi.org/10.1088/1367-2630/11/4/043032

[81] Eibenberger, S., Gerlich, S., Arndt, M., Mayor, M., Tüxen, J.: Matter–wave interference of particles selected from a molecular library with masses exceeding 10 000 amu. Physical Chemistry Chemical Physics **15**(35), 14696 (2013) https://doi.org/10.1039/c3cp51500a

[82] Fein, Y.Y., Geyer, P., Zwick, P., Kiałka, F., Pedalino, S., Mayor, M., Gerlich, S., Arndt, M.: Quantum superposition of molecules beyond 25 kda. Nat. Phys. **15**, 1242–1245 (2019) https://doi.org/10.1038/s41567-019-0663-9
